# Supplementary material for: DB-PAISA: Discovery-Based Privacy-Agile IoT Sensing+Actuation
Source: arXiv:2412.11572 source file (2024-12-16)
Supplement: Supplementary file 1 [file 99-appendix_detailed.tex]

\appendix

\newpage

\section{\paisaplus Variant -- \private \label{sec:inventory}}

\begin{figure}[t]
  \centering
  \captionsetup{justification=centering}
  \includegraphics[width=0.95\columnwidth]{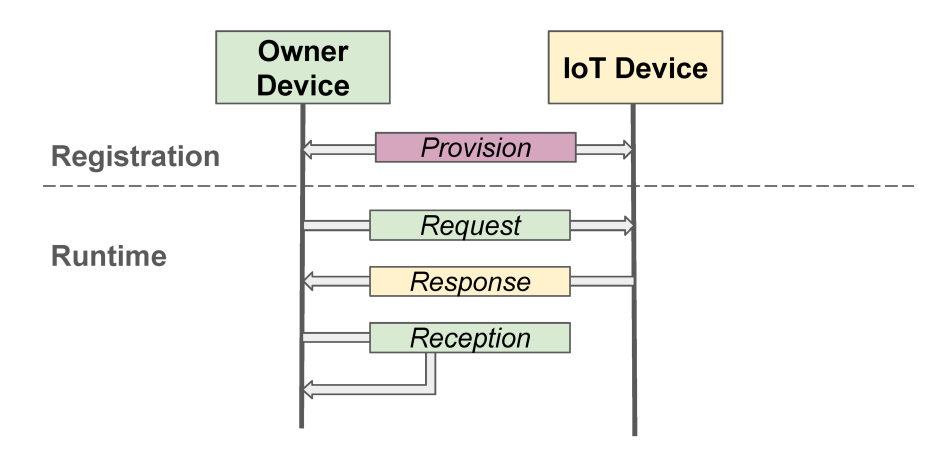}
  \vspace{-0.3cm}
  \caption{\private Overview}
  \label{fig:inventory}
  \vspace{-0.4cm}
\end{figure}

\private has two components: \ownerdev and \iotdev. \ownerdev is the owner's device authorized to 
solicit information from a multitude of \iotdev-s in a large industrial setting.
As shown in Figure \ref{fig:inventory}, \private also has two phases: {\it Registration} and {\it Runtime}.

\noindent {\bf $\boldsymbol{\registration}$ phase} occurs prior to device deployment.
Each \iotdev is securely provisioned with (1) unique secret key (\seckey) shared with \ownerdev, 
(2) its own device information, and (3) \ownerdev's public key (\ownerpk).

\noindent {\bf $\boldsymbol{\runtime}$ phase} has three steps: \request, \response, and \receptionusr.
There are three significant differences from \pub: (1) \requestmessage is authenticated with 
\ownerdev's private key (\ownersk), (2) \responsemessage is encrypted with \seckey, and
(3) \attest takes place upon every \requestmessage.

\noindent {\em NOTE:} Due to space constraints, implementation and evaluation of \private are not present in this work.
Nonetheless, we fully implemented it at \cite{paisaplus-code}.

\subsection{\private Adversary model} \label{subsec:inventory-adv}
\noindent {\bf DoS attacks on \iotdev-s:}
Similar to \pub, malware \sadv can try to deplete \iotdev resources via software vulnerabilities.
However, DoS attacks from a network \sadv are more challenging to address because of costly
verification of \ownerdev's signatures in \requestmessage-s.
Potential mitigation techniques are discussed in Section \ref{subsec:discussion-dos}.

\noindent {\bf Replay attacks:}
A network-based \sadv can replay arbitrary messages to both \ownerdev and \iotdev-s.

\noindent {\bf Eavesdropping:}
A network-based \sadv can eavesdrop on all \private protocol messages to learn
individual \iotdev information and the number and types of deployed \iotdev-s.
\sadv can also attempt to link occurrences of one or more \iotdev-s.

\subsection{\private Requirements}
\noindent{\bf System requirements:} are the same as in \pub, except that scaling to multiple users is no longer a concern in \private.
Although \private operates in settings with large numbers of \iotdev-s, only an authorized \ownerdev can solicit information from them.

\noindent{\bf Security requirements (beyond those of \pub):}
\begin{compactitem}
    \item {\it Request authentication:} \iotdev must validate each \requestmessage.
    \item {\it Response confidentiality:} \responsemessage must not leak information about \iotdev.
    \item {\it Unlinkability:} Given any two valid \responsemessage-s, the probability of determining if they were produced by the same \iotdev should be negligibly close to 50\%, for any party except \ownerdev.
\end{compactitem}

\subsection{\private Protocol Details} \label{subsec:inventory_detail}
In this section, we only describe the aspects of \private that differ from \pub.
Figures \ref{fig:prot-inv-reg} and \ref{fig:prot-inv-runtime} summarize \registration and \runtime phases, respectively.

\subsubsection{Registration}
\ownerpk, \seckey, and some metadata are securely installed for each \iotdev. However, information 
that is not deployment-dependent (such as \privatetcb, \iotdevsofthash, and peripheral configuration) 
are assumed to be securely provisioned earlier by \mfr. 
Note that, since \ownerdev is aware of all identities and types of its \iotdev-s, there is no 
longer any need for either {\bf $\boldsymbol{\devmanifest}$} or {\bf $\boldsymbol{\devmanifesturl}$}.
As a result, \mfr plays no active role in \private.
The {\bf TCB} of \private is identical to that of \pub.

\begin{figure}[t]
  \centering  
  \captionsetup{justification=centering}  
  \includegraphics[height=1.8in,width=0.95\columnwidth]{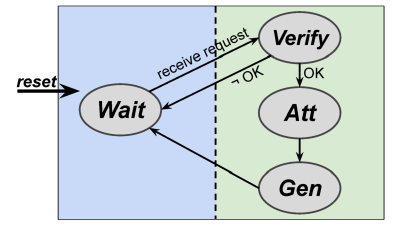}
  \vspace*{-.3cm}  
  \caption{\private State Machine on \iotdev}
  \label{fig:inventory_state_machine}
  \vspace*{-0.35cm}
\end{figure}

\subsubsection{Runtime} \label{subsubsec:inventory-runtime}
Similar to \pub, the \private \runtime phase has three steps: \request, \response, and \receptionusr.

\paragraph{\bf $\boldsymbol{\privatetcb}$ on $\boldsymbol{\iotdev}$: }
As discussed in Section \ref{subsec:inventory-adv}, DoS attacks by a network-based \sadv are out-of-scope.
Also, scalability is not an issue since only one \ownerdev is assumed.
Furthermore, because \ownerdev's requests are expected to be much less frequent 
than \usrdev's requests in \pub, \attest is performed on the fly upon each \ownerdev's request.

Figure \ref{fig:inventory_state_machine} shows four state machines of \iotdev:

\noindent{\bf (a) $\boldsymbol{\wait}$:}
The only transition is switching to $\boldsymbol{\verifystep}$ when \requestmessage is received.

\noindent{\bf (b) $\boldsymbol{\verifystep}$:}
\iotdev verifies \requestmessage with \ownerpk.
If verification succeeds, it transitions to $\boldsymbol{\attest}$.
Otherwise, it discards \requestmessage and returns to $\boldsymbol{\wait}$.

\noindent{\bf (c) $\boldsymbol{\attest}$:}
\iotdev computes \attestresult and transitions to $\boldsymbol{\gen}$.
Note that \iotdev need not compute attestation time because \attest occurs with every \requestmessage, thus $\attestreport := [\attestresult]$.

\noindent{\bf (d) $\boldsymbol{\gen}$:}
\iotdev encrypts \noncevalue{\owner}{} (\ownerdev's nonce in \requestmessage), device information (e.g., \iotdevid, \iotdev type, 
\iotdevsoft version), and \attestreport with \seckey, i.e., $\encvalue{\resp} := \encfunc(\seckey, \noncevalue{\owner}{}||\attestreport||\text{device information})$, where \encfunc\ is an encryption operation.
It composes \responsemessage containing an authentication tag, e.g., using AES-CCM/GCM.
Since \responsemessage is encrypted, multiple \responsemessage-s from the same \iotdev are
unlinkable as long as: (1) \seckey is not leaked, (2) \seckey is sufficiently long and randomly
chosen, and (3) the underlying symmetric encryption algorithm is secure.
However, we acknowledge that address information in packet headers of \responsemessage-s 
can be used to track \iotdev. We discuss how to address this problem in 
Appendix \ref{subsection:appendix-discussion}.

\paragraph{\bf $\boldsymbol{\private}$ app on $\boldsymbol{\ownerdev}$: }
There are two steps on \ownerdev: \request and \receptionusr.

\noindent{\bf \request:} \ownerdev signs \noncevalue{\owner}{} with \ownersk \ and broadcasts \requestmessage, containing \noncevalue{\owner}{} and the signature (\sigvalue{\req}).
After sending \requestmessage, it starts a scan to receive \responsemessage-s from potential nearby \iotdev-s.

\noindent{\bf \receptionusr:}
Upon receiving \responsemessage, \ownerdev retrieves the corresponding \seckey in brute-force attempts, i.e., it attempts to decrypt \requestmessage with all \seckey-s.
This demands O($n$) computations on \ownerdev, where $n$ is the number of \iotdev.
Its overhead and alternative approaches are discussed in Section \ref{sec:discussion-key-retrieval}.
After retrieving \seckey, it decrypts it with the \seckey, and finally, details are displayed on \ownerdev.

\subsection{Discussion} \label{subsection:appendix-discussion}
\noindent {\bf $\boldsymbol{\requestmessage}$ DoS Mitigation:}
Mitigating DoS attacks in \private is more challenging. The lazy-response technique used in \pub is
unsuitable for \private because each \requestmessage requires individual verification and response.
One radical approach is to skip verification of \requestmessage-s altogether.
This way, \iotdev inundated with \requestmessage-s would generate as many 
\responsemessage-s. However, symmetric encryption of \responsemessage-s is much
less expensive than signature verification of \requestmessage-s.
Also, lack of \requestmessage authentication would allow a network-based \sadv to generate
fake \requestmessage-s and harvest replies.
Although \sadv would not be able to track individual \iotdev-s, it can easily learn {\em the number} of nearby \iotdev-s.

Another alternative is using Lamport's hash chains \cite{lamport1981} to authenticate \requestmessage-s.
While inexpensive, hash chains prompt well-known synchronization issues, plus the need to support a separate
(and robust) hash chain renewal mechanism.

\noindent {\bf $\boldsymbol{\iotdev}$ Unlinkability of $\boldsymbol{\responsemessage}$-s:}
As mentioned earlier, if a network-based \sadv learns that multiple \responsemessage-s 
are emitted by the same \iotdev, it can effectively track that it.

As discussed in Section \ref{sec:inventory}, all fields in \responsemessage 
are encrypted and \seckey is presumably never leaked, sufficiently long (bit-wise), and
randomly selected. Also, the underlying symmetric encryption algorithm is secure.
Furthermore, all \responsemessage-s must be of uniform size, regardless of the type/model
of the responding \iotdev. Therefore, we can rule out linkability based on analysis of 
\responsemessage payloads.

However, the BLE packet header format includes certain static fields, such as the MAC address and UUID.
\iotdev can be trivially tracked by observing these fields in multiple BLE packets \cite{bello2019privacy}.
Fortunately, BLE supports MAC address randomization to prevent tracking \cite{ludant2021linking}.
Randomization can be done periodically (e.g., daily or hourly) or based on an event (e.g., per packet).
Although this raises some performance issues (such as connection un-pairing, 
MAC address change overhead), \iotdev in \private can randomize the MAC address per \responsemessage.
We believe this is acceptable since \ownerdev is expected to issue requests relatively infrequently. 
Finally, to prevent UUID-based tracking, we insert a random UUID into every \requestmessage header.

\section{\private Protocol Details} \label{sec:private-prot}
\private protocol (i.e., \registration and \runtime phases) is depicted in detail in Figures \ref{fig:prot-inv-reg} and \ref{fig:prot-inv-runtime}.

\begin{figure}[H]
  \captionsetup{justification=centering}
  \begin{tcolorbox} [standard jigsaw, opacityback=0.3]
      \begin{protocol}
      \footnotesize
      \registration phase of \private is consists of one procedure, \provision, and is specified as follows: \\
          
          \begin{compactenum} []
              \item {\textcolor{blue-violet}{\provision} $[\ownerdev \longrightarrow \iotdev]$:} \\
              Let (\ownerpk, \ownersk) be \ownerdev key-pair.
              \private software (\privatetcb) and a hash of device software (\iotdevsofthash) are assumed to be embedded before \provision by \mfr.
              
              \ownerdev generates $T$ as per equation \ref{eq:T-enroll} and installs $T$ inside \iotdev secure region.
                  \begin{equation}\label{eq:T-enroll}
                  \begin{split}
                     T := (\ownerpk||\seckey||\iotdevsofthash)
                  \end{split}
                  \end{equation}
                  , where \seckey is a shared-key with \ownerdev.
              \end{compactenum}
      \end{protocol}
  \end{tcolorbox}
  \vspace{-.4cm}
  \caption{\private \ \registration Phase}
  \label{fig:prot-inv-reg}
  \vspace{-.4cm}
\end{figure}

\begin{figure}[H]
  \captionsetup{justification=centering}
  \begin{tcolorbox} [standard jigsaw, opacityback=0.5]
      \begin{protocol}
        \footnotesize
        \private\ \runtime phase is consist of three steps: \request, \response, and \receptionusr. Akin to \pub, \usrdev carries out \request and \receptionusr steps, while \iotdev handles \response step. \\

        \textcolor{blue-violet}{\response} $[\iotdev \circlearrowright]$:
        \iotdev has four states: \wait, \verify, \attest, and \gen. 
        
        \begin{compactenum}[]
            \item \textcolor{applegreen}{\wait} $[\iotdev \circlearrowright]$ : \\
                Upon boot with initiated secure timer, \iotdev starts listening for \requestmessage-s.
                When \requestmessage is received and identified with \private protocol identifier \privateid, it proceeds to \verify.
                
            \item \textcolor{applegreen}{\verifystep} $[\iotdev \circlearrowright]$ : \\
                Verifies signature \sigvalue{\req} in \requestmessage with \ownerpk.
                It the verification fails, it discards \requestmessage. Otherwise, it proceeds to \attest.
                
            \item \textcolor{applegreen}{\attest} $[\iotdev \circlearrowright]$ :                
                \begin{compactenum}
                    \item Measures \iotdevsoft\ and assigns $\attestresult := \{\verb+Success+\}$ if $\hashfunc(\iotdevsoft) == \iotdevsofthash$. Otherwise, $\attestresult = \{\verb+Fail+\}$.
                    \item Proceeds to \gen.
                \end{compactenum}
            \item \textcolor{applegreen}{\gen} $[\iotdev \circlearrowright]$ :
                \begin{compactenum}
                    \item Generates \encvalue{\resp}:
                    \begin{equation}\label{eq:enc-resp}
                        \begin{split}
                            \encvalue{\resp} := \encfunc(\seckey, \attestreport||\text{device information})
                        \end{split}                         
                    \end{equation}
                    Device information may include \iotdevid, \iotdev type, and \iotdevsoft version.
                    \item Composes: \\
                    $\responsemessage := \{\encvalue{\resp}\}$
                    \item Broadcasts \responsemessage.
                \end{compactenum}
                
        \end{compactenum}
        \ \\

        \usrdev performs two steps: \request and \receptionusr.
          
        \begin{compactenum}[]
            \item { \textcolor{blue-violet}{\request} $[\ownerdev \longrightarrow \iotdev]$:} \\
            \ownerdev broadcasts an authenticated request as follows:
            \begin{compactenum}
                \item Generates a signature \sigvalue{\req}:
                \begin{equation}\label{eq:sig-req}
                    \sigvalue{\req} := \sigfunc(\ownersk, \noncevalue{\owner}{})
                \end{equation}
                \item Composes \requestmessage and broadcasts it: \\
                $\requestmessage := \{\noncevalue{\owner}{}, \sigvalue{\req}, \privateid\}$.
            \end{compactenum}            
            
            \item { \textcolor{blue-violet}{\receptionusr} $[\ownerdev \circlearrowright]$:}
            Upon reception of \responsemessage from \iotdev, \ownerdev follows:
            \begin{compactenum}
                \item Validates and decrypts \responsemessage with \seckey.
                If the validation fails, it aborts and outputs $\perp$ [\responsemessage tampering/forging].
                \item If \noncevalue{\owner}{} is not in \responsemessage, it aborts and outputs $\perp$ [replay attack].
                \item Outputs (\devmanifest, \attestreport).
            \end{compactenum}
        \end{compactenum}
        
    \end{protocol}
\end{tcolorbox}
\vspace{-.4cm}
\caption{\private \ \runtime Phase}
\label{fig:prot-inv-runtime}
\vspace{-.4cm}
\end{figure}

% \section{Extended Discussion \& Limitations}\label{sec:extended_limitation}
%

\begin{figure}[t]
  \centering  
  \captionsetup{justification=centering}  
  \includegraphics[width=0.95\columnwidth]{img/mac_computation.pdf}
  % \vspace*{-.3cm}
  \vspace*{-.3cm} 
  \caption{Key Retrieval Overheads on \ownerdev (Na\"ive Approach)}
  \label{fig:mac-computation}
  % \vspace*{-0.35cm}
\end{figure}

\begin{figure}[t]
  \centering  
  \captionsetup{justification=centering}  
  \includegraphics[width=0.95\columnwidth]{img/LKH.pdf}
  \vspace*{-.3cm}    
  \caption{Key Tree in Logical Key Hierarchy (LKH)}
  \label{fig:key-tree}
  % \vspace*{-0.35cm}
\end{figure}

\begin{table}[b]
\captionsetup{justification=centering}
\vspace*{.2cm}
\resizebox{0.95\columnwidth}{!}{%
    \begin{tabular}{?c|c?c|c|c?}
    \thickhline
    \rowcolor{yellow!5}
    {\bf Device} & {\bf Overheads} & {\bf {\makecell{Na\"ive \\ Approach}}} & {\bf {\makecell{LKH with \\ Binary Tree}}} & {\bf {\makecell{LKH with \\ Non-Binary Tree}}} \\
    \thickhline
    \cellcolor{yellow!5} & \cellcolor{yellow!5} Computation & -- & $O(\log n)$ & $O(\log_p n)$ \\ \cline{2-5}
    \cellcolor{yellow!5} & \cellcolor{yellow!5} Key Storage & -- & $\log n$ & $2*n$ \\ \cline{2-5}
    \cellcolor{yellow!5} \multirow{-3}{*}{$\boldsymbol{\iotdev}$} & \cellcolor{yellow!5} \responsemessage size & -- & $\log n*y$ & $\log_p n*y$ \\ \thickhline
    \cellcolor{yellow!5} & \cellcolor{yellow!5} Computation & $O(n)$ & $O(\log n)$ & $O(p*\log_p n)$ \\ \cline{2-5}
    \cellcolor{yellow!5} \cellcolor{yellow!5} \multirow{-2}{*}{$\boldsymbol{\ownerdev}$} & \cellcolor{yellow!5} Key Storage & $n$ & $2*n ^*$ & ${\frac{pn}{p-1}} ^*$ \\ \thickhline
    \multicolumn{5}{l}{\small * Holds as $n$ is large enough.} \\
    \end{tabular}
}
\vspace*{.3cm}
\caption{Key Retrieval Overhead Comparisons \\
            ($n$: the number of \iotdev-s,\ $y$: PRF output size)}
\label{table:comparison-key-retrieval}
% \vspace*{-.6cm}
\end{table}

\section{\private Key Retrieval on \ownerdev} \label{sec:discussion-key-retrieval}
Recall that in \private,  \responsemessage is encrypted with \seckey using symmetric encryption.
To decrypt given \responsemessage, \ownerdev must identify unique \seckey corresponding to \iotdev.
% The key retrieval process is quite tricky in order to guarantee \responsemessage without revealing any identifiable information.
Note that \iotdev's \responsemessage should not contain any identifiable information about \iotdev to prevent a trace of \iotdev.

As a na\"ive approach, \ownerdev can decrypt \responsemessage using a brute-force approach:
\ownerdev finds \seckey by validating an authentication tag in \responsemessage with all keys.
While inefficient, this is not infeasible in practice; according to \verb|Crypto++ 5.6.0| library (open-source) benchmark \cite{crypto++},
GMAC (in AES-GCM) takes 3.2 cycles per byte and CMAC (in AES-CCM) takes 16.1 cycles per byte.
Assuming \ownerdev runs at 2.0 GHz, checking a key for \responsemessage (20 bytes) takes up to 32 ns and 161 ns, respectively.
As shown in Figure \ref{fig:mac-computation}, \ownerdev can successfully brute-force find \seckey in 32 ms (AES-GCM) with a million of \iotdev-s.

Another efficient means is utilizing Logical Key Hierarchy (LKH) for key retrieval \cite{wong2000secure}.
LKH is an efficient and scalable solution to address key management in secure hierarchical group communication.
It constructs a key tree as shown in Figure \ref{fig:key-tree}, where each leaf node represents an \iotdev.
The height of the tree, denoted by $L$, is $\ceil{\log n}$, where $n$ is the number of \iotdev-s in the system.
Each \iotdev has $L$ or $L-1$ keys, depending on its level.
For example, Dev$_k$ in Figure \ref{fig:key-tree} has $K_{k,0}$, $K_{k,1}$, ..., $K_{k,L}$ keys.
While LKH is originally designed for key-sharing between leaf nodes in a tree, we additionally involve \ownerdev who possesses all $K_{i,j}$ shared with Dev$_i$-s.

Note that keys in intermediate nodes are shared with all their descending \iotdev-s.
For example, in level $L-1$, $K_{0, L-1}$ is shared by Dev$_0$ and Dev$_1$, i.e., $K_{0, L-1} = K_{1, L-1}$.
In level $L-2$, $K_{0, L-2}$ is shared by Dev$_0$, Dev$_1$, Dev$_2$, and Dev$_3$.
$K_{0, 0}$ in the root node is shared by all \iotdev-s.
To generalize this, $K_{i,j}$ remains identical, shared between Dev$_i$-s, where $i$ $\in$ [$\floor{i/k}*k, (\floor{i/k}+1)*k-1]$ and $k = 2^{(L-j)}$.

Given the keys shared in a hierarchy, we now describe how to generate untraceable \responsemessage.
Each Dev$_i$ prepends a header for secure identification to ${\responsemessage}_{_i}$, composing ${\responsemessage}'_{_i}$ as below:
$$
\responsemessage'_{_i} = [\mathcal{F}_{K_{i, 1}}(\noncevalue{\owner}{}) \ || \ ... \ || \ \mathcal{F}_{K_{i, L}}(\noncevalue{\owner}{}) \ || \ \responsemessage_{_i}]
$$
where $\mathcal{F}$ is a pseudorandom function (PRF) $\mathcal{F}: \mathcal{K} \times \mathcal{X} \rightarrow \mathcal{Y}$.
For a random key $k \in \mathcal{K}$, $\mathcal{F}$ is indistinguishable from a uniformly random function.
Consequently, \ownerdev can identify Dev$_i$ as follows:
\begin{enumerate}[(1)]
    \item Computes $\mathcal{F}_{K_{0, 1}}(\noncevalue{\owner}{})$ with \noncevalue{\owner}{}, contained in \requestmessage.
    \item If it matches with $\mathcal{F}_{K_{i, 1}}(\noncevalue{\owner}{})$ in ${\responsemessage}'_{_i}$, it goes to the left child node. Otherwise, it goes to the right child node.
    \item Computes $\mathcal{F}_{K_{m, l}}(\noncevalue{\owner}{})$, where $m$ is the left child index and $l$ is its level.
    \item If it matches with $\mathcal{F}_{K_{i, l}}(\noncevalue{\owner}{})$ in ${\responsemessage}'_{_i}$, it goes to the left child node. Otherwise, it goes to the right child node.
    \item Repeat (3)-(4) until it reaches the leaf node, $K_{k, L}$ (or $K_{k, L-1}$). 
    \item \ownerdev identifies \iotdev Dev$_k$, and decrypts ${\responsemessage}_{_i}$ with \seckey.
\end{enumerate}

For example, consider key retrieval for ${\responsemessage}'_{_2}$ generated by Dev$_2$,
${\responsemessage}'_{_2}$ = $[\mathcal{F}_{K_{2, 1}}(\noncevalue{\owner}{}) \ || \ ... \ || \ \mathcal{F}_{K_{2, L}}(\noncevalue{\owner}{}) \ || $
$ \ \responsemessage_{_i}]$.
To identify the key used for $\responsemessage_{_i}$ encryption, \ownerdev must determine the path from the root node to the leaf node in Figure \ref{fig:key-tree} as follows.
\ownerdev checks if the first field of the header, $\mathcal{F}_{K_{2, 1}}(\noncevalue{\owner}{})$, is the same as $\mathcal{F}_{K_{0, 1}}(\noncevalue{\owner}{})$ in level 1.
Since it matches, it goes to the left child node, $\mathcal{F}_{K_{0, 2}}(\noncevalue{\owner}{})$ in level 2.
Then, \ownerdev checks if the $l$-th field of the header, $\mathcal{F}_{K_{2, l}}(\noncevalue{\owner}{})$, is identical to $\mathcal{F}_{K_{0, l}}(\noncevalue{\owner}{})$ in level $l$.
As it matches until level $L-3$, the left child nodes are selected.
In level $L-2$, it does not match; it goes to the right child node.
In level $L-1$, it matches with ($\mathcal{F}_{K_{2, L-1}}(\noncevalue{\owner}{})$); hence, it goes to the left child,
and finally, it reaches $K_{2, L}$. Therefore, \ownerdev concludes that ${\responsemessage}_{_i}$ comes from Dev$_2$ and decrypts it with Dev$_2$'s \seckey.

% \begin{enumerate}[(1)]
%     \item \ownerdev checks if the first field of the header, $\mathcal{F}_{K_{2, 1}}(\noncevalue{\owner}{})$, is the same as $\mathcal{F}_{K_{0, 1}}(\noncevalue{\owner}{})$ in level 1.
%     \item Since it matches, it goes to the left child node, $\mathcal{F}_{K_{0, 2}}(\noncevalue{\owner}{})$ in level 2.
%     \item \ownerdev checks if the $l$-th field of the header, $\mathcal{F}_{K_{2, l}}(\noncevalue{\owner}{})$, is the same as $\mathcal{F}_{K_{0, l}}(\noncevalue{\owner}{})$ in level $l$.
%     \item As it matches until level $L-3$, left child nodes are selected.
%     \item In level $L-2$, it does not match; it goes to the right child node.
%     \item In level $L-1$, it matches with ($\mathcal{F}_{K_{2, L-1}}(\noncevalue{\owner}{})$), hence, it goes to the left child.
%     \item It reaches $K_{2, L}$. Therefore, \ownerdev concludes that \responsemessage comes from Dev$_2$.
% \end{enumerate}

Note that $K_{0,0}$ is not used as it is shared across all \iotdev-s, and thus indistinguishable.
Whereas, $K_{i, L}$ can be adopted as \seckey for Dev$_i$ because it is shared only between Dev$_i$ and \ownerdev.

The na\"ive approach requires $O($n$)$ computation while \ownerdev needs only $O(L)$ computation to identify Dev$_i$ as Dev$_k$.
However, LKH demands more secure storage on each \iotdev to store $L$ keys.
It also increases the size of \responsemessage$'$ by $L*y$, where $y$ is the output size of $\mathcal{F}$.
Meanwhile, \ownerdev needs to store $\approx 2*n$ keys, where $n$ is sufficiently large.

To further reduce the runtime overhead of LKH, \ownerdev can pick a larger number, $p$, as a base of the logarithm function.
In this case, $L = \log_p n$, where $n$ is the number of \iotdev-s.
Then, \ownerdev computes up to $p-1$ times to decide the path in each level $l$ as follows:
$\mathcal{F}_{K_{m+q, l}}(\noncevalue{\owner}{})$, where $q \in [0, p-1]$.
As a result, it demands for \ownerdev to compute $(p-1)*L$. 
This reduces \responsemessage$'$ size from $\log n + \mathcal{E}$ to $L + \mathcal{E}$, where $\mathcal{E}$ is the size of \responsemessage.
Also, \ownerdev should store $\frac{pn}{p-1}$ keys, where $n$ is sufficiently large.
The comparison is summarized in Table \ref{table:comparison-key-retrieval}.

In conclusion, \ownerdev is capable of decrypting \responsemessage without identifiable information leakage using either brute-force attempts or LKH with tradeoffs for each.
